# Supplementary material for: TopSpace: spatial topic modeling for unsupervised discovery of multicellular spatial tissue structures in multiplex imaging
Source: arXiv:2504.18495 ancillary file (2025-04-25)
Supplement: Supplementary file 1 [file Suppl-TopSpace.pdf]

# Supplementary material for TopSpace: spatial topic modeling for unsupervised discovery of multicellular spatial tissue structures in multiplex imaging

Junsouk Choi, Jian Kang, and Veera Baladandayuthapani

2025-04-21

# Contents


**Introduction** **5**

**1 Methodology** **7**
- 1.1 TopSpace notations . . . 7
- 1.2 Posterior computation . . . 7
- 1.3 Selection of the number of topics $K$ . . . 10
- 1.4 A high-resolution version of Figure 1 . . . 11

**2 Simulation studies** **13**
- 2.1 Simulation scenarios . . . 13
- 2.2 Modified squared exponential kernel . . . 15
- 2.3 Evaluation metrics . . . 15
- 2.4 A high-resolution version of Figure 2 . . . 16

**3 Analysis of NSCLC data** **19**
- 3.1 Quantitative imaging features . . . 19
- 3.2 Cox regression using quantitative imaging features . . . 20
- 3.3 A high-resolution version of Figure 3 . . . 21

# Introduction

Recent development of multiplex imaging technologies such as cyclic immunoflourescene (CyCIF), CO-Dectection by indEXing (CODEX), multiplex immunohistochemistry (mIHC), and multiplex ion beam imaging (MIBI) allows for measuring the expression of tens of protein markers at single-cell resolution while preserving spatial information of cells. This enables spatially resolved understanding of cellular heterogeneity and organization within tissues. Compared to conventional single-cell sequencing technologies, multiplex imaging provides unique opportunities to examine higher-order spatial patterns in tissue architecture and characterize specific tissue microenvrionments, which hold systematic implications for disease pathology and clinical outcomes. To support and facilitate the analysis of spatial tissue architecture in multiplex tissue imaging data, we propose TopSpace, a novel Bayesian spatial topic model for unsupervised learning of high-level spatial structures of tissues that may be potential determinant of patient outcomes.

This is a supplementary file for the paper titled "TopSpace: spatial topic modeling for unsupervised discovery of multicellular spatial tissue structures in multiplex imaging". The contents of the supplementary file is outlined below.

A) In Section 1, we present an additional description about our proposed TopSpace, including the detailed steps for its MCMC implementation.
B) Further details of the simulation studies are discussed in Section 2.
C) Additional findings from the analysis of non-small cell lung cancer data are provided in Section 3.

# Chapter 1

# Methodology

## 1.1 TopSpace notations

In the TopSpace framework, we treat each individual cell in a multiplex image as a "word" in the traditional topic modeling paradigm, with the various cell types forming the "word vocabulary". Local neighborhoods—distinct segments of the entire multiplex image—are considered as "documents", where the positions of these neighborhoods are known. In this context, the "topics", inferred by our TopSpace method, represent multicellular microenvironments where specific cell types co-localize. Table 1.1 provides detailed descriptions of the notations used in TopSpace.

## 1.2 Posterior computation

For posterior inference on the proposed TopSpace, we develop a computationally efficient MCMC algorithm to simulate its posterior distribution. Specifically, to improve scalability of our posterior computation procedure, we adopt a basis expansion of the GP priors in light of the eigendecomposition of the covariance kernel. With a sufficiently large set of eigenfunctions, the proposed TopSpace can be well approximated by a truncated linear combination of eigenfunctions, allowing us to develop a Metropolis-Hastings within Gibbs sampling algorithm in an efficient manner.

### 1.2.1 GP prior representation

Consider the eigendecomposition of the covariance kernel $\kappa(s, s') = \sum_{l=1}^{\infty} \lambda_l \phi_l(s)\phi_l(s')$, where $\{\lambda_l\}_{l=1}^{\infty}$ is the set of eigenvalues with $\lambda_1 \geq \cdots \geq \lambda_l \geq \lambda_{l+1} \geq \cdots$, and $\{\phi_l(s)\}_{l=1}^{\infty}$ is the set of orthonormal eigenfunctions

Table 1.1: Description of the TopSapce notations.

| Notation | Description |
|---|---|
| $K$ | number of topics |
| $H$ | number of cell types |
| $M$ | number of local neighborhoods |
| $N_i$ | number of cells in the $i$-th local neighborhood |
| $s_i$ | spatial coordinates of the $i$-th neighborhood |
| $x_{i(j)}$ | cell type of the $j$-th cell in the $i$-th neighborhood |
| $z_{i(j)}$ | topic assignment for the $j$-th cell in the $i$-th neighborhood |
| $\beta_k$ | discrete distribution of cell types for the $k$-th topic |
| $\alpha_i$ | discrete distribution of topics for the $i$-th neighborhood |
| $\theta(s_i)$ | spatially varying hyperparameter for the Dirichlet prior on $\alpha_i$, which depend on $s_i$ |
| $\gamma$ | hyperparameter for the Dirichlet prior for $\beta_k$ |
| $\kappa$ | covariance kernel for the Gaussian process prior on $\log(\theta_k(\cdot))$ |

such that $\int \phi_l(s)\phi_{l'}(s)ds = 1(l = l')$ for any $l, l' \in \{1, 2, \ldots\}$. The Karhunen–Loève theorem implies that $\log \theta_k(\cdot) \sim \mathcal{GP}(0, \kappa(\cdot, \cdot))$ can be represented as a linear combination of the eigenfunctions, $\log \theta_k(\cdot) = \sum_{l=1}^{\infty} b_{kl}\psi_l(\cdot)$, where $\psi_l(\cdot) = \sqrt{\lambda_l}\phi_l(\cdot)$ and $b_{kl} \overset{i.i.d.}{\sim} \mathrm{N}(0, 1)$. In practice, we can truncate this summation at a sufficiently large finite number of components $L$ to obtain a fairly good approximation of $\log \theta_k(s)$: $\log \theta_k(s) \approx \sum_{l=1}^{L} b_{kl}\psi_l(s)$. Since the topic distributions across local neighborhoods are assumed to be spatially smooth, the required number of eigenfunctions $L$ to achieve a good approximation of $\log \theta_k(\cdot)$ is still much smaller than the number of neighborhoods $M$. Therefore, with this approximation, the number of parameters for inferring $\log \theta_k(\cdot)$ can be reduced substantially, leading to an efficient posterior computation.

### 1.2.2 Markov chain Monte Carlo

With the approximated GP prior on $\log \theta_k$, we develop a Metropolis-Hastings within Gibbs sampling algorithm to draw samples from the posterior distribution of TopSpace. For $\beta_k$ and $\alpha_i$, the full conditional distributions have the closed form, leading to the Gibbs sampling update schemes. For $z_{i(j)}$, we use the collapsed Gibbs sampling, marginalizing out $\beta_k$ and $\alpha_i$ from our target posterior distribution. Updating the basis coefficients $B = (b_{kl})_{k,l}$, which approximate the GP priors, is the most challenging step due to its high-dimensionality and the complexity of the full conditional density involving the log transformation. Therefore, we adopt the stochastic gradient Hamiltonian Monte Carlo (Chen et al., 2014) to update $B$ given the other parameters. The detailed steps of our Metropolis-Hastings within Gibbs sampler for our TopSpace are as follows:

#### 1.2.2.1 Update $Z$

For $i = 1, \ldots, M$, $j = 1, \ldots, N_i$, we sample $z_{i(j)}$ from its conditional posterior $Pr(z_{i(j)} = \tilde{k} | Z \setminus \{z_{i(j)}\}, B, X)$, marginalizing out $\beta$ and $\alpha$, where

$$Pr(z_{i(j)} = \tilde{k} | Z \setminus \{z_{i(j)}\}, B, X) \propto \frac{n^{(-ij)}_{\tilde{k}x_{ij}} + \gamma_{x_{ij}}}{\sum_{h=1}^{H}(n^{(-ij)}_{\tilde{k}h} + \gamma_h)} \frac{N^{(-ij)}_{i\tilde{k}} + \theta_{\tilde{k}}(s_i)}{\sum_{k=1}^{K}(N^{(-ij)}_{ik} + \theta_k(s_i))}. \tag{1.1}$$

Here, $n_{kh}$ denotes the number of times cell type $h$ is assigned to topic $k$ and $N_{ik}$ denotes the number of cell types in neighborhood $i$ assigned to topic $k$. The superscript $(-ij)$ indicates that the corresponding cell has been disregarded when calculating $n_{kh}$ and $N_{ik}$.

#### 1.2.2.2 Update $\beta$

For $k = 1, \ldots, K$, we sample $\beta_k$ from its full conditional

$$\pi(\beta_k | Z, X) \propto \text{Dirichlet}\left(n_{k1} + \gamma_1, \ldots, n_{kH} + \gamma_H\right). \tag{1.2}$$

#### 1.2.2.3 Update $\alpha$

We sample $\alpha_i, i = 1, \ldots, M$, from their full conditionals

$$\pi(\alpha_i | Z, B, X) \propto \text{Dirichlet}\left(N_{i1} + \theta_1(s_i), \ldots, N_{iK} + \theta_K(s_i)\right). \tag{1.3}$$

#### 1.2.2.4 Update B

The full conditional distribution of the basis coefficents $B$, which approximate the GPs over $\log \theta_k(\cdot)$, is given by

$$\pi(B | \alpha, X) \propto \prod_{i=1}^{M} \frac{1}{\mathrm{B}\left(\theta_1(s_i), \ldots, \theta_K(s_i)\right)} \alpha_{i1}^{\theta_1(s_i)-1} \cdots \alpha_{iK}^{\theta_K(s_i)-1} \prod_{k=1}^{K} \prod_{l=1}^{L} \exp\left(-\frac{1}{2} b_{kl}^2\right), \tag{1.4}$$

where $\mathrm{B}\left(\theta_1(s_i), \ldots, \theta_K(s_i)\right)$ is the beta function with $\theta_k(s_i) = \exp\left(\sum_{l=1}^{L} b_{kl}\phi_l(s_i)\right)$. It is infeasible to directly sample $B$ from (1.4); therefore, we use the stochastic gradient Hamiltonian Monte Carlo (Chen et al., 2014) to draw samples of $B$. Hamiltonian Monte Carlo (Neal, 2011) is an efficient MCMC sampling approach which shows a higher acceptance rate compared to the standard Metropolis-Hastings sampling. SGHMC extends HMC by using stochastic gradients to improve efficiency, allowing it to avoid evaluating the entire dataset. Additionally, SGHMC eliminates the need for the Metropolis-Hastings step after each proposal by introducing an additional friction term in the momentum update. Specifically, at $t$-th MCMC iteration, we update $B$ as follows:

- Initialize $(B_0, r_0) = (B^{(t-1)}, r^{(t-1)})$.

- Optionally, re-sample momentum $r$ from the matrix normal distribution $r \sim MN_{K\times L}(0, I, \eta I)$.
- For $h = 1, \ldots, H$, repeat:
  - Update $B_h = B_{h-1} + r_{h-1}$.
  - Sample $\varepsilon_h \sim MN_{K\times L}(0, I, 2\alpha\eta I)$.
  - Subsample the indices of local neighborhoods $\mathcal{I} \subset \{1, \ldots, M\}$.
  - Update $r_h = (1-\alpha)r_{h-1} - \eta\nabla\tilde{U}(B_h; \mathcal{I}) + \varepsilon_h$, where $\nabla\tilde{U}(B_h; \mathcal{I}) = \left(\frac{\partial\tilde{U}(B)}{\partial b_{kl}}\right)_{k,l}$ is the stochastic gradient of $U(B) = -\log\pi(B|\alpha, X)$, with each partial derivative given by

$$\frac{\partial\tilde{U}(B)}{\partial b_{kl}} = \frac{M}{|\mathcal{I}|}\sum_{i\in\mathcal{I}}\left\{\psi\left(\theta_k(s_i)\right) - \psi\left(\sum_{k=1}^{K}\theta_k(s_i)\right) - \log(\alpha_{ik})\right\}\theta_k(s_i)\phi_l(s_i) + b_{kl}. \tag{1.5}$$

- Update $(B^{(t)}, r^{(t)}) = (B_H, r_H)$.

Here, $H, \eta$, and $\alpha$ are the hyperparameters for SGHMC, which represent the number of leapfrog steps, the learning rate, and the friction term, respectively.

## 1.3 Selection of the number of topics $K$

Determining the number of topics $K$ in topic modeling is often challenging, particularly for multiplex imaging data where domain knowledge alone often cannot accurately specify the number of tissue microenvironments. If the number of topics is too small, the model becomes too simplistic and fails to capture the complex biological structures in tissues. Conversely, if the number of topics is too large, the model becomes excessively complex, potentially leading to overfitting. Therefore, identifying an optimal $K$ is crucial for the effective performance of our TopSpace.

We use the deviance information criterion (DIC) to determine the optimal number of topics $K$ from the data. Calculating DIC involves computing the log-likelihood for each posterior sample, and we specifically use the observed-data likelihood from the TopSpace model, as suggested previously in Li et al. (2020). Using the observed-data likelihood rather than the conditional likelihood helps avoid theoretical complications associated with applying DIC to latent variable models such as LDA. The DIC for our TopSpace model is then given by

$$\text{DIC} = p_D + \overline{D(\beta, \alpha)}, \tag{1.6}$$

where the deviance is defined as

$$D(\beta, \alpha) = -2\sum_{i=1}^{M}\sum_{j=1}^{N_i}\log\left\{\sum_{k=1}^{K}\sum_{h=1}^{H}1(x_{i(j)} = h)\alpha_{ik}\beta_{kh}\right\}$$

and $p_D = \frac{1}{2}\overline{\text{Var}(D(\beta, \alpha))}$ denotes the effective number of parameters of the model (Gelman et al., 1995).

## 1.4 A high-resolution version of Figure 1

Schematics of the TopSpace workflow. (A) TopSpace input data. TopSpace takes as input a multiplex image that includes individual cell phenotypes and predefined local neighborhoods. (B) A schematic representation of the TopSpace generative process. TopSpace leverages spatial GPs to account for spatial dependencies in the composition of tissue microenvironments (topics) across local neighborhoods. By analyzing co-occurrence of different cell types within these local neighborhoods while incorporating spatial information, TopSpace identifies latent tissue microenvironments (topics) characterized by unique distributions of cell types. (C) Spatial tissue structure identification using TopSpace. The results inferred by TopSpace are utilized to determine the spatial distribution of tissue microenvironments.

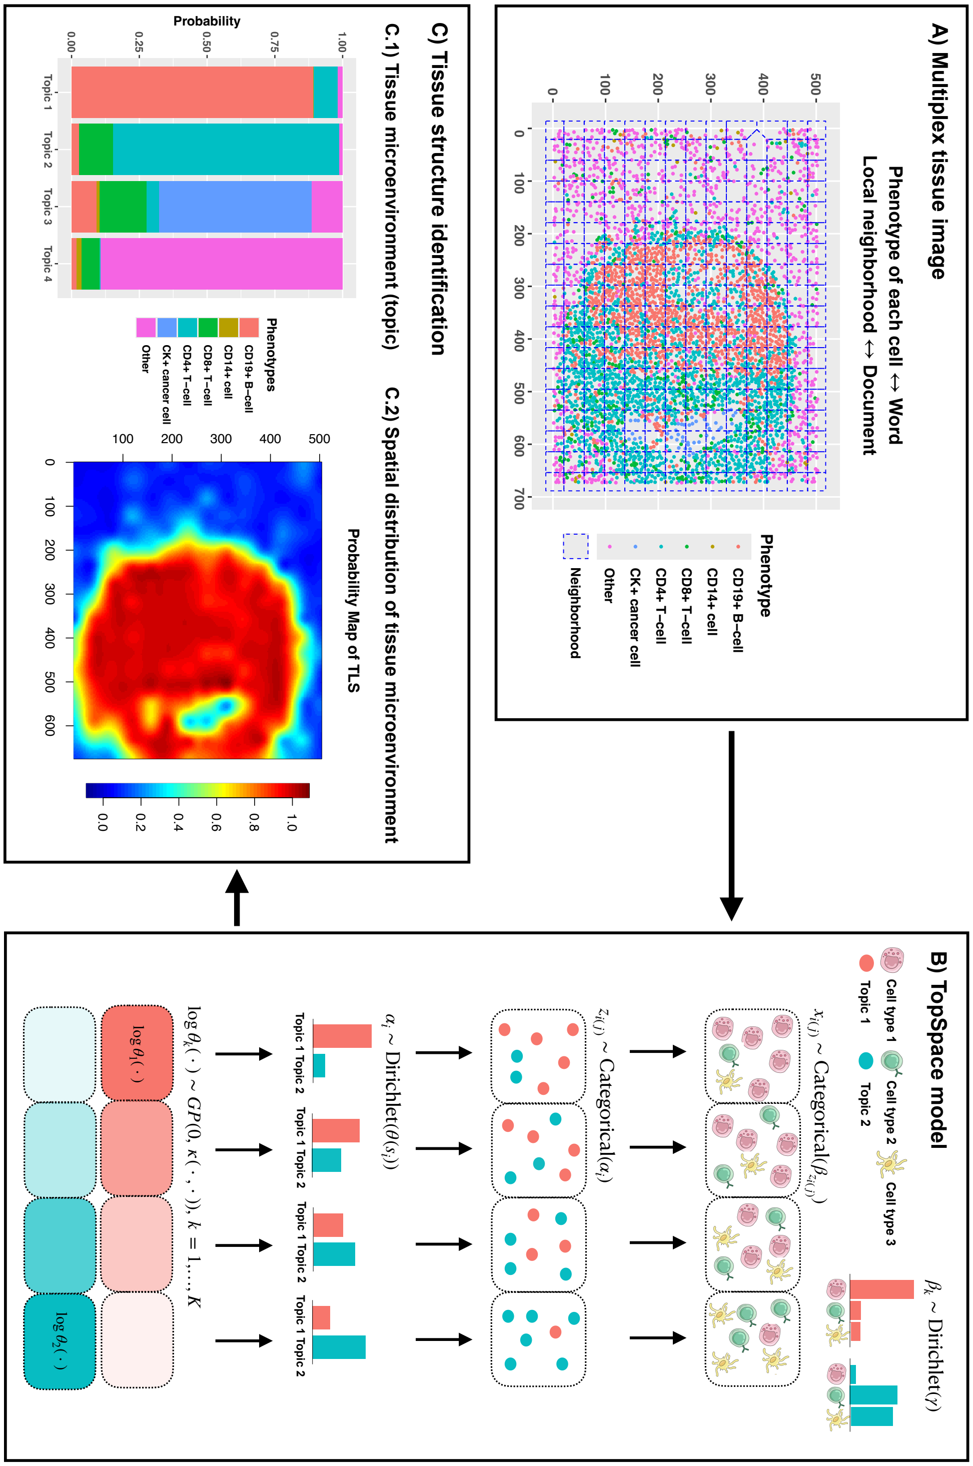
A) Multiplex tissue image
Phenotype of each cell ↔ Word
Local neighborhood ↔ Document
Phenotype
CD19+ B−cell
CD14+ cell
CD8+ T−cell
CD4+ T−cell
CK+ cancer cell
Other
Neighborhood
B) TopSpace model
Cell type 1
Cell type 2
Cell type 3
Topic 1
Topic 2
$\beta_k \sim \text{Dirichlet}(\gamma)$
$x_{i(j)} \sim \text{Categorical}(\beta_{z_{i(j)}})$
$z_{i(j)} \sim \text{Categorical}(\alpha_i)$
$\alpha_i \sim \text{Dirichlet}(\theta(s_i))$
$\log \theta_k(\cdot) \sim GP(0, \kappa(\cdot,\cdot)), k = 1,\ldots,K$
$\log \theta_1(\cdot)$
$\log \theta_2(\cdot)$
C) Tissue structure identification
C.1) Tissue microenvironment (topic)
Probability
Topic 1
Topic 2
Topic 3
Topic 4
Phenotypes
C.2) Spatial distribution of tissue microenvironment
Probability Map of TLS

# Chapter 2

# Simulation studies

In this section, we provide additional details regarding the simulation studies in the main manuscript.

## 2.1 Simulation scenarios

We generated a synthetic tissue image consisting of $M = 441$ local neighborhoods, each centered on evenly spaced grid points within the plane $[-1, 1]^2$ at 0.1 intervals. For each neighborhood, we placed $N_i = 10$ cells—consistent with the median cell count per neighborhood in the multiplex images of the NSCLC dataset (Section 4)—resulting in a total of 4,410 cells. We considered $H = 6$ cell types, aligning with those in the NSCLC dataset, and assumed the presence of $K = 3$ latent topics. With per-topic cell type distributions sampled from the Dirichlet distribution, $\beta_k \sim \text{Dirichlet}(0.2)$, the phenotype of each cell was generated using the proposed TopSpace model, where we employed the modified squared exponential kernel as the covariance kernel $\kappa$ for the GP prior on $\log \theta_k$.

The modified squared exponential covariance kernel includes two hyperparameters $a$ and $b$, where $a$ is the decay parameter regulatingthe rate of variance decay of the GP, while $b$ represents the smoothing parameter controlling the smoothness of the GP and thereby influencing spatial correlations between locations. A smaller value of $b$ results in a smoother process, yielding increased spatial dependency. The exact definition of the modified squared exponential kernel is provided below. For our experiments, we fixed $a = 0.01$ and varied $b \in \{5, 1, 0.2\}$ to induce three levels of spatial correlations, denoted $S_{low}$, $S_{med}$, and $S_{high}$, respectively. Specifically, at the 10th percentile of pairwise distances between neighborhoods, the spatial correlation of $\log \theta_k(s)$ was 0.427, 0.844, and 0.967 for the low ($S_{low}$), medium ($S_{med}$), and high ($S_{high}$) spatial correlation scenarios. Figure 2.1 illustrates how spatial correlation varies with distance under each scenario.

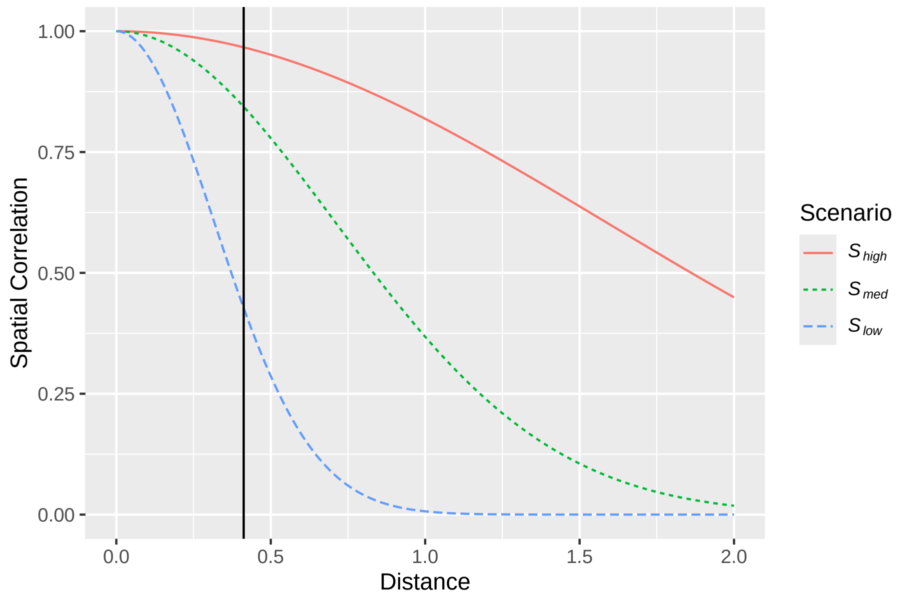


Figure 2.1: The spatial correlation $\rho_b(d) = \exp\{-bd^2\}$ of $\log\theta_k(s_i)$ and $\log\theta_k(s_{i'})$ at distance $||s_i - s_{i'}||_2 = d$. We consider three spatial correlation levels $b \in \{5, 1, 0.2\}$: low ($S_{low}$), medium ($S_{med}$), and high ($S_{high}$). The black vertical line indicates the spatial correlation at the 10th percentile of pairwise neighborhood distances.

## 2.2 Modified squared exponential kernel

In our simulation studies, we used the modified squared exponential covariance kernel for the GP over $\log \theta_k(\cdot)$, defined as

$$\kappa(s_i, s_{i'}) = \exp\{-a(||s_i||_2^2 + ||s_{i'}||_2^2) - b||s_i - s_{i'}||_2^2\}, \tag{2.1}$$

where $||\cdot||_2$ denotes the Euclidean norm, and $a > 0$ and $b > 0$ are hyperparameters. When $\log \theta_k(\cdot)$ follows a GP with mean zero and the modified squared exponential covariance kernel, the hyperparameter $a$ controls the rate at which the variance $\text{Var}\{\log \theta_k(\cdot)\}$ decays relative to $\text{Var}\{\log \theta_k(\mathbf{0})\}$. Meanwhile, the hyperparameter $b$ determines the smoothness of the process; smaller values of $b$ result in smoother Gaussian processes. An important advantage of using the modified squared exponential kernel is that its eigenfunctionscan be easily constructed using the Hermite polynomials, thereby facilitating our posterior computation discussed in Section 2.3.

## 2.3 Evaluation metrics

We evaluated the methods in Section 3 using two primary metrics. First, to measure how well each method recovers latent topics, we computed the total Kullback–Leibler (KL) divergence between true and estimated topics $\beta_k$'s, $\sum_{k=1}^{K} \text{KL}(\beta_k||\hat{\beta}_k)$, where

$$\text{KL}(\beta_k||\hat{\beta}_k) = \sum_{h=1}^{H} \beta_{kh} \log\left(\frac{\beta_{kh}}{\hat{\beta}_{kh}}\right).$$

Next, to evaluate spatial clustering performance, we used the adjusted rand index (ARI) between true and estimated clustering memberships, where the neighborhoods in the synthetic imaging data were clustered based on their dominant topics inferred by each method. The ARI (Hubert and Arabie, 1985) is defined by

$$\text{ARI} = \frac{\sum_{ij}\binom{M_{ij}}{2} - \left[\sum_i \binom{A_i}{2} \sum_j \binom{B_j}{2}\right] \Big/ \binom{M}{2}}{\frac{1}{2}\left[\sum_i \binom{A_i}{2} + \sum_j \binom{B_j}{2}\right] - \left[\sum_i \binom{A_i}{2} \sum_j \binom{B_j}{2}\right] \Big/ \binom{M}{2}},$$

where $M$ is the total number of local neighborhoods, $M_{ij}$ is the number of neighborhoods where the estimated dominant topic is $i$ and the true dominant topic is $j$, $A_i$ is the total number of neighborhoods with the estimated dominant topic $i$, and $B_j$ is the total number of neighborhoods with the true dominant topic $j$. The ARI ranges from 0 to 1, with 1 indicating perfect agreement between the estimated and true clusterings (here, dominant topics), and 0 corresponds to random assignments.

## 2.4 A high-resolution version of Figure 2

Comparison of the performance of TopSpace, LDA, and spLDA in identifying latent topics and performing spatial clustering across simulation scenarios with different degrees of spatial dependencies. spLDA was fitted using various values for the tuning parameter $d_{ij}$, which regulates the strength of spatial coherence among adjacent neighborhoods. (A) Boxplots of the total KL divergence between true and estimated $\beta_k$'s, $\sum_{k=1}^{K} \mathrm{KL}(\beta_k||\hat{\beta}_k)$, for each method, calculated across 50 replicates under varying degrees of spatial dependencies $S_{low}$, $S_{med}$ and $S_{high}$. (B) Boxplots of ARIs comparing true and estimated spatial clustering for TopSpace, LDA, and spLDAs across 50 replicates under different spatial dependency scenarios.

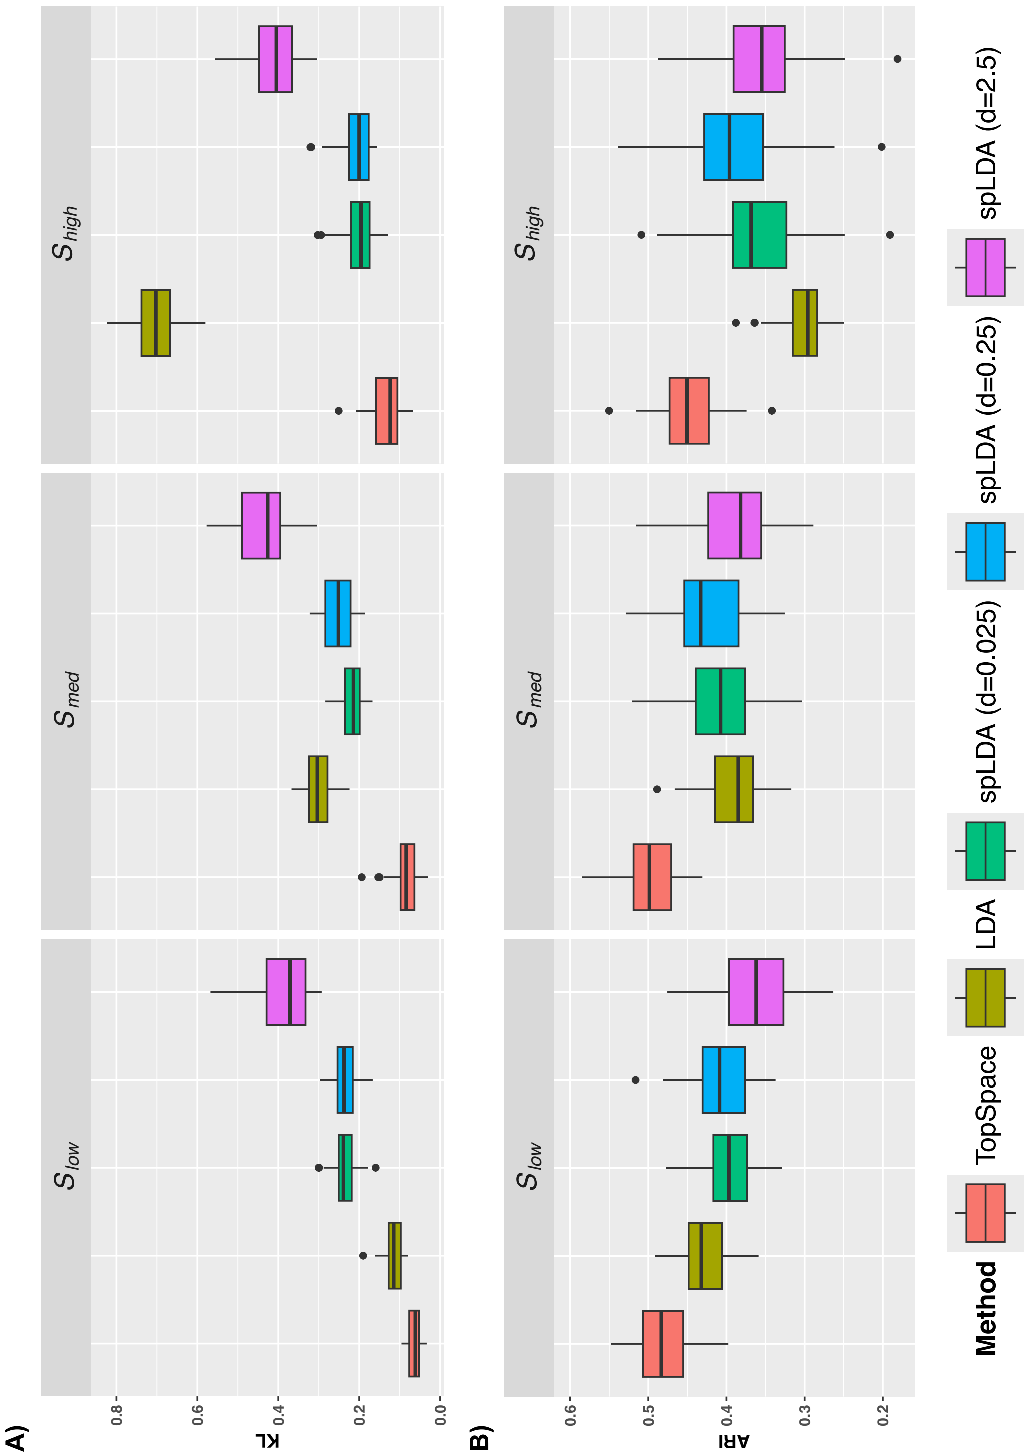
A)
KL
0.8
0.6
0.4
0.2
0.0
$S_{low}$
$S_{med}$
$S_{high}$
B)
ARI
0.6
0.5
0.4
0.3
0.2
Method
TopSpace
LDA
spLDA (d=0.025)
spLDA (d=0.25)
spLDA (d=2.5)

# Chapter 3

# Analysis of NSCLC data

In this section, we present additional findings from our study of the non-small cell lung cancer (NSCLC) dataset, including survival analysis results using quantitative imaging features.

## 3.1 Quantitative imaging features

In our analysis of the NSCLC dataset, we computed two quantitative imaging features from the spatial probability map of tertiary lymphoid structure (TLS). Specifically, we calculated two widely-used radiomics features, energy and entropy, to quantify the spatial distribution patterns of TLS, thereby providing insight into tissue heterogeneity and its potential prognostic implications.

For a multiplex tissue image, let $p(s_i)$ denote the probability of TLS at neighborhood location $s_i$ within the spatial probability map of TLS. Then, energy and entropy were calculated as follows:

- **Energy**:

$$Energy = \sum_{i=1}^{M} (p(s_i))^2.$$

  Energy measures the overall magnitude of TLS probabilities in a multiplex tissue image. A larger values implies a greater sum of the squares of the TLS probabilities.

- **Entropy**:

$$Entropy = -\sum_{b=1}^{B} H(b) \log_2 H(b),$$

  where $H$ is the histogram that divides the TLS probabilities $p(s_i)$ into $B$ equally spaced bins. Entropy measures the inherent uncertainty/randomness in the TLS distribution in the tissue section. The

maximum value of entropy occurs when all the probability values of TLS in a multiplex image occur with equal probability.

These features provide quantitative measures of the spatial distribution of TLS, beyond the simple identification of their presence or absence. By incorporating both energy and entropy, we are able to capture different aspects of TLS distribution, offering a more comprehensive view of the immune landscape within the tumor microenvironment.

## 3.2 Cox regression using quantitative imaging features

We performed a Cox proportional hazards regression analysis to examine the association between patient survival and the radiomics features derived from the TLS spatial probability maps. For each radiomics feature, we fitted a Cox regression model adjusted for other clinical variables—patient age and tumor stage. The results of the analysis are summarized in 3.1:

Table 3.1: Cox regression results based on the quantitative imaging features.

| Predictor | Hazard Ratio | 90% Confidence Interval | p-value |
|---|---|---|---|
| *Energy* | 0.996 | (0.991, 1.002) | 0.200 |
| *Entropy* | 0.922 | (0.855, 0.992) | 0.069 |

Entropy, which measures the randomness or heterogeneity in TLS distribution, was found to be significant in our Cox survival analysis, with the estimated hazard ratio of 0.922 (90% CI: 0.855 to 0.992, p-value = 0.069), where we used a lenient significance level $\alpha = 0.1$, reflecting the challenge of limited sample size of the NSCLC dataset. Higher randomness/heterogeneity in TLS distribution was associated with better survival outcomes. This suggests that a highly heterogeneous TLS distribution may reflect an active immune environment capable of mounting effective responses against tumor progression, which contributes to improved patient prognosis. On the other hand, energy was not found to be significant with a p-value above the significance level of 0.1. While this implies that energy is not a strong survival predictor within the scope of our NSCLC dataset, it still provides valuable insights into the overall magnitude of TLS distribution and may be relevant for other aspects of immune response characterization. Further research may be needed to determine whether energy could hold predictive value for different clinical outcomes.

Our Cox regression analysis demonstrates the prognostic utility of TLS quantification based on the spatial probability map generated by our TopSpace approach. The clinical relevance of this tissue structure quantification might be further validated through additional investigations involving larger, independent cohorts.

## 3.3 A high-resolution version of Figure 3

Analysis of the non-small cell lung cancer dataset collected from 153 patients. (A) Representative images displaying 6 cell types, with colors specified in the legend. (B) Estimated topics (per-topic cell type distributions) and spatial clustering based on dominant topics, achieved through the application of TopSpace to the representative images. Selection of the number of topics was guided by the DIC, choosing four topics for the first image and five for the second. Topics are arranged to highlight specific microenvironments, with Topic 1 representing the B-cell zone and Topic 2 (as well as Topic 3 for the second image) representing the T-cell zone. (C) The spatial probability map of TLS for each image, created by combining probabilities of Topics 1 and 2 (and Topic 3 for the second image) across local neighborhoods. Areas in red and blue depict high and low probabilities of TLS, respectively. (D) Kaplan-Meier survival curves for patients with and without TLS. (E) Boxplots comparing survival days between patients with and without TLS, using data from uncensored patients only; significant difference indicated by the p-value of 0.007 from the Wilcoxon test.

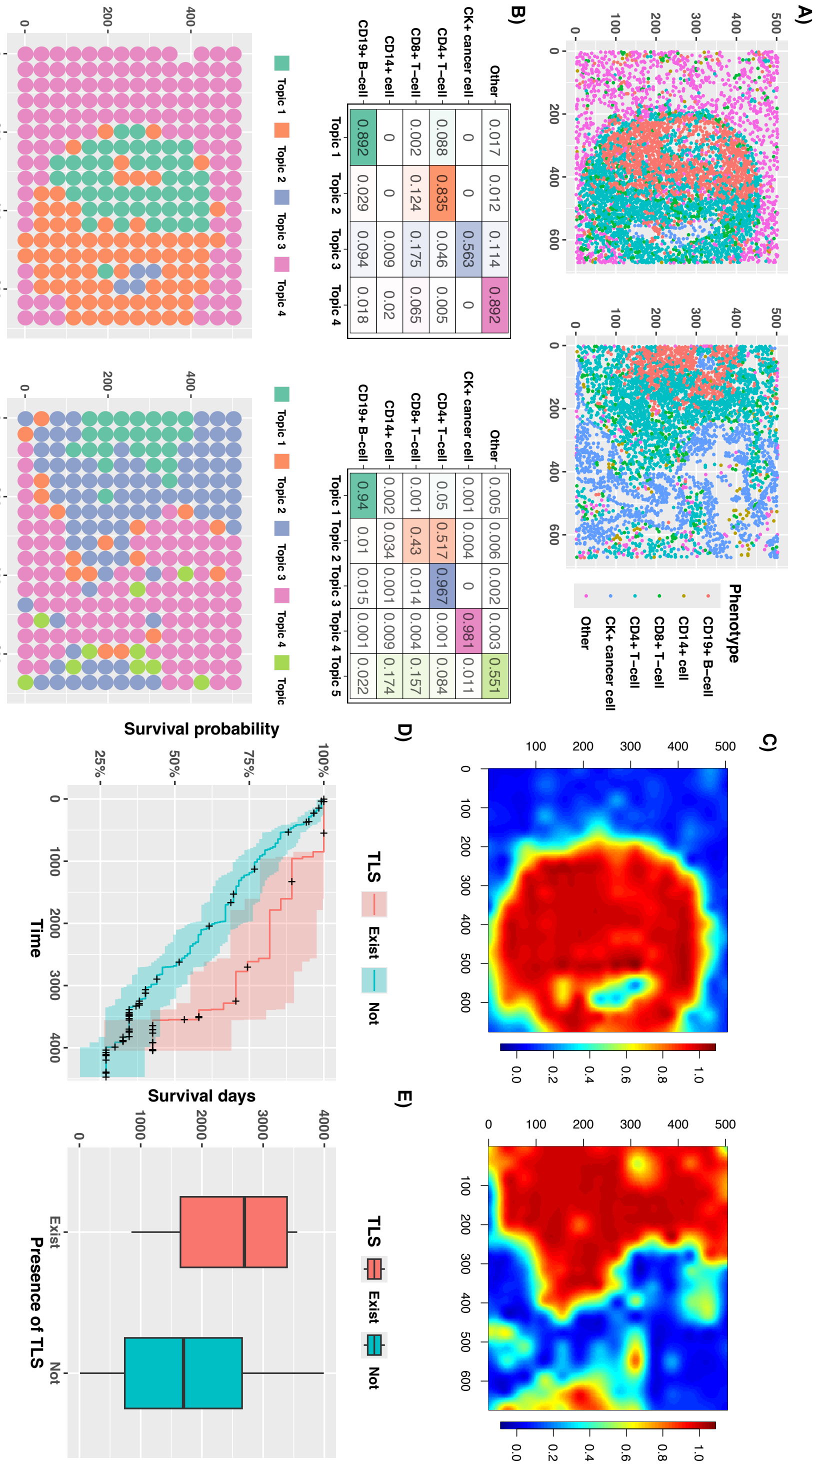
A)
Phenotype
CD19+ B−cell
CD14+ cell
CD8+ T−cell
CD4+ T−cell
CK+ cancer cell
Other
B)
Topic 1
Topic 2
Topic 3
Topic 4
C)
D)
TLS
Exist
Not
Survival probability
Time
E)
Survival days
Presence of TLS

# Bibliography


Chen, T., Fox, E., and Guestrin, C. (2014). Stochastic gradient hamiltonian monte carlo. In Xing, E. P. and Jebara, T., editors, *Proceedings of the 31st International Conference on Machine Learning*, volume 32 of *Proceedings of Machine Learning Research*, pages 1683–1691, Bejing, China. PMLR.

Gelman, A., Carlin, J. B., Stern, H. S., and Rubin, D. B. (1995). *Bayesian Data Analysis*. Chapman & Hall/CRC Texts in Statistical Science. Chapman & Hall/CRC, Philadelphia, PA.

Hubert, L. and Arabie, P. (1985). Comparing partitions. *J. Classif.*, 2(1):193–218.

Li, Y., Yu, J., and Zeng, T. (2020). Deviance information criterion for latent variable models and misspecified models. *J. Econom.*, 216(2):450–493.

Neal, R. (2011). MCMC using hamiltonian dynamics. In *Chapman & Hall/CRC Handbooks of Modern Statistical Methods*. Chapman and Hall/CRC.
